# Supplementary material for: Extending Basic Block Versioning with Typed Object Shapes
Source: arXiv:1507.02437 source file (2015-07-09)
Supplement: Supplementary file 1 [file againstsm_decr_sm_baseline.tex]

-267
