# Supplementary material for: Extending Basic Block Versioning with Typed Object Shapes
Source: arXiv:1507.02437 source file (2015-07-09)
Supplement: Supplementary file 2 [file againstsm_decr_sm_no_inlining.tex]

44
